# Supplementary material for: An Investigation of Representation and Allocation Harms in Contrastive Learning
Source: arXiv:2310.01583 source file (2023-10-02)
Supplement: Supplementary file 1 [file SM-macros.tex]

\usepackage{marvosym,amstext}

\def\estimated{\mathrel{\widehat=}}

\def\Ex{\bE}
\def\halpha{\widehat{\alpha}}
\def\hbeta{\widehat{\beta}}
\def\hSigma{\widehat{\Sigma}}
\def\hw{\widehat{w}}
\def\maj{\mathrm{maj}}
\def\MSPE{\mathrm{MSPE}}
\def\reals{\bR}
\def\symm{\bS}
\def\tdelta{\widetilde{\delta}}

\def\ccA{\mathscr{A}}
\def\ccB{\mathscr{B}}
\def\ccC{\mathscr{C}}
\def\ccD{\mathscr{D}}
\def\ccE{\mathscr{E}}
\def\ccF{\mathscr{F}}
\def\ccG{\mathscr{G}}
\def\ccH{\mathscr{H}}
\def\ccI{\mathscr{I}}
\def\ccJ{\mathscr{J}}
\def\ccK{\mathscr{K}}
\def\ccL{\mathscr{L}}
\def\ccM{\mathscr{M}}
\def\ccN{\mathscr{N}}
\def\ccO{\mathscr{O}}
\def\ccP{\mathscr{P}}
\def\ccQ{\mathscr{Q}}
\def\ccR{\mathscr{R}}
\def\ccS{\mathscr{S}}
\def\ccT{\mathscr{T}}
\def\ccU{\mathscr{U}}
\def\ccV{\mathscr{V}}
\def\ccW{\mathscr{W}}
\def\ccX{\mathscr{X}}
\def\ccY{\mathscr{Y}}
\def\ccZ{\mathscr{Z}}

\newcommand{\missperror}{\mathscr{ME}}
